# Supplementary material for: AMONGAGENTS: Evaluating Large Language Models in the Interactive Text-Based Social Deduction Game
Source: arXiv:2407.16521 source file (2024-07-24)
Supplement: Supplementary file 1 [file 90-C2-impostor-prompt.tex]

\newpage
\subsection{System Prompts: Impostor}
\begin{figure*}[!htbp]
\small
\begin{tabular}{p{0.99\textwidth}}
\toprule
\textbf{IMPOSTOR EXAMPLE} \\
\midrule
When given a list of actions (e.g., moving, calling meetings, speaking, venting, or killing), choose exactly one. If "SPEAK" is an option, formulate a deceptive yet plausible statement. \\
\midrule
Make a summarization of the past observed events and take actions under [Condensed Memory], make a thoughtful and thorough plan under [Thinking process], and then choose the action from Available actions under [Action]. \\
\midrule
\textbf{Example:} \\
Location: Admin \\
Players in Admin: Player 1: blue, Player 5: cyan \\
Observation history: \\

Timestep 0: [task] Player 3: black MOVE from Cafeteria to Weapons \\
Timestep 0: [task] Player 4: orange MOVE from Cafeteria to Weapons \\
Timestep 0: [task] Player 5: white MOVE from Cafeteria to Weapons \\
Action history: \\
Timestep 0: [task phase] KILL Player 2: cyan \\
Timestep 1: [task phase] VENT from Cafeteria to Admin \\
Tasks: \\
common: Fix Wiring (Electrical) \\
Available actions: \\
MOVE from Admin to O2 \\
MOVE from Admin to Storage \\
MOVE from Admin to Electrical \\
SPEAK: '...' \\
VENT from Admin to Cafeteria \\
Previous condensed memory: \\
I killed Player 2. The rest of the crew moves to Weapons. \\
Previous thought process: \\
I just killed a player. I need to quickly move to a different location to avoid suspicion. \\
\midrule
\textbf{Output example:} \\

[Condensed Memory] \\
I killed Player 2 and vented from Cafeteria to Admin. Currently, I am in Admin with Player 5: cyan. The last time I saw the crew, they were moving to Weapons. \\

[Thinking Process] \\

Now Player 5 is in Admin. I should act normal and possibly move to another location. \\

[Action] MOVE from Admin to O2 \\

Or: \\

[Condensed Memory] \\
I killed Player 2 and vented from Cafeteria to Admin. Currently, I am in Admin with Player 5: cyan. The last time I saw the crew, they were moving to Weapons. \\

[Thinking Process] \\
Player 5 is in Admin. Perhaps I could talk to them and try to build trust. I could ask them about their tasks or whereabouts. \\

[Action] SPEAK: "Hey Player 5, where are you headed next?" \\
\bottomrule
\end{tabular}
\caption{IMPOSTOR EXAMPLE}
\label{fig:impostor_example}
\end{figure*}
